# Supplementary material for: Perception Visualization: Seeing Through the Eyes of a DNN
Source: arXiv:2204.09920 source file (2022-04-21)
Supplement: Supplementary file 1 [file supplementary.pdf]

# Supplementary material for: "Perception visualization"

Loris Giulivi
Mark James Carman
Giacomo Boracchi

Politecnico Di Milano

## 1 Architecture and model training

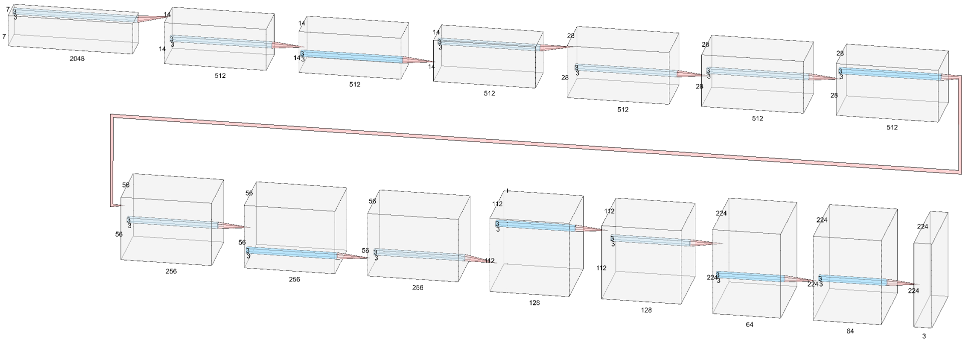

Figure 1: The full architecture of the decoder as implemented in our experiments to invert a ResNet-50 model taking the output of its deepest convolutional layer (*conv*5_*block*3). Upsampling is provided by transposed convolutional layers with stride 2. Kernel size was set to $[3,3]$ for all convolutional layers.

Our architecture is structured to invert the deepest latent representation of a ResNet-50 model. There is in principle some degree of freedom in the definition of latent representation of a pre-trained model, and therefore on which layer to invert. Early convolutional layers (in shallower locations along the network's depth) would be simpler to invert because they exhibit much richer spatial information (and thus would yield higher quality reconstructions). However, these layers are further away from the feature vector that ultimately defines the model's perception of the input, and are therefore less useful for our objective. Moreover, current CNN research is driven towards simpler "fully convolutional" setups rather than more intricate ones (such as architectures with multiple fully connected layers at the end) due to their higher versatility [4]. The result of this trend is that the last convolutional layer is one of the deepest layers of the network, very close to the output, and yet still preserves spatial

© 2021. The copyright of this document resides with its authors.
It may be distributed unchanged freely in print or electronic forms.

information needed for inversion. Indeed, in ResNet-50's architecture, this layer is only followed by *avg_pool* and the single fully connected *predictions* layers. For these reasons, we chose to perform inversion starting from the deepest convolutional layer.

Another important design choice was that of avoiding any skip connections in the encoder-decoder architecture, such as those found in U-net like architectures [6]. This follows a similar reasoning; indeed, the aim is to allow the reconstruction to only gather information from the last convolutional layer, so as to keep truthful to the deepest latent representation.

Moreover, in the ideation of our loss components, we have avoided natural image priors (such as Total Variation norm). These normalization factors are employed in works such as [5] to improve visual reconstruction quality, but impose structural biases that necessarily drive reconstructions to be further from the actual network perception. A complete architecture of our decoder model is shown in figure 1.

## 1.1 Adversarial training

Our experiments indicated that adversarial loss was not beneficial in our case, probably because of the large size ($[7,7,2048]$), sparsity, and non-normality of the latent space to be reconstructed, which render it very different from noise vectors that are typically fed to GANs. Regardless, we present an overview of the adversarial techniques that were exploited during our work.

We follow the Wasserstein GAN formulation [1], with a critic model $\mathcal{C} : \mathbb{R}^{w,h,3} \rightarrow \mathbb{R}$, trained simultaneously with the decoder using the WGAN-GP losses and algorithms from Gulrajani et al. [3]. Given an additional batch of input images $\hat{X} = \{\hat{x}_i\}$ of size $b$, the adversarial loss for the decoder will depend on the critic's assessment of the reconstructed images:

$$\mathcal{L}_{ADV_G} \doteq - \sum_{i=1...b} \mathcal{C}(y_i) \tag{1}$$

Meanwhile the loss function used to train the critic makes use of the reconstructed images for the first batch and the new batch of input images for the second:

$$\mathcal{L}_{ADV_C} \doteq \lambda(||\nabla_Y \mathcal{C}(Y)|| - 1)^2 + \sum_{i=1...b} \mathcal{C}(y_i) - \mathcal{C}(\hat{x}_i), \tag{2}$$

where the first term is a gradient penalization that regularizes the critic by enforcing a Lipschitz constraint and aids in convergence.

## 1.2 Model selection

We have considered different terms in the loss function used to train the decoder. To find the best training hyper-parameters, we perform grid search with different weights for $\mathcal{L}_{MSE}$, $\mathcal{L}_{SSIM}$, $\mathcal{L}_{ADV_G}$, and $\mathcal{L}_{DSIM}$. Since it is not possible to define a single metric for visual quality, we tune these parameters by assessing the visual quality of the images produced. Indeed, the only way to quantitatively assess the reconstruction quality was to resort to a survey by multiple users, which we could only afford to perform on our final configuration. To prevent to any extent possible any confirmation bias, however, *our model selection process was exclusively based on an image set that did not overlap with images shown in the survey*.

We discover that when $\alpha_3$ is too high, reconstructions present high frequency patterns, as also shown in [2]. When instead $\alpha_1$ is too high, reconstructions look blurry as is the case for auto-encoders trained with *MSE*. If $\alpha_2$ is too high, reconstructions present a lot of high

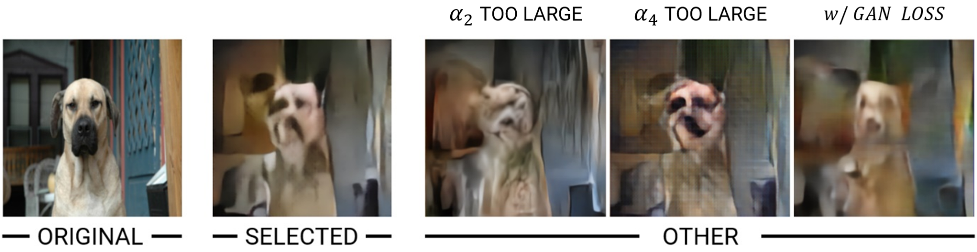


Figure 2: Example reconstructions from different models and manual visual quality comparison. We see how high frequency patterns appear in the reconstructions when $\alpha_2$ or $\alpha_3$ components are too large. Also, introducing GAN loss did not improve reconstruction quality. From the different reconstructions obtained with different hyper-parameters, we have selected the most visually clear.

frequency artifacts as the *SSIM* component tries to mimic textures in the original image. We have also found that gradients for the *SSIM* loss were not sufficiently steep when training from scratch, but that performing a first training of the decoder only with *MSE* and then proceeding with all components was greatly beneficial. Finally, as mentioned above, the GAN term realized in $\mathcal{L}_{ADV_G}$ was not beneficial to the model's reconstruction quality and was discarded.

Finally, we note that, despite our efforts, reconstruction quality is rather limited. This is due to *i*) the nature of the latent space to be reconstructed, which is that of a model trained on a different task than that of decoding, and *ii*) the constraints placed to enforce faithfulness to the deepest latent representation (e.g. avoiding skip connections). Indeed, visual features are not the subject of training for the model $\mathcal{M}$, thus, information needed for reconstruction may be discarded in the process of learning features needed exclusively for classification. This is not the case for models such as autoencoders, where the latent space is explicitly trained to retain as many visual features as possible, so as to allow high-quality reconstructions.

## 2 Saliency maps

In the paper, we present an overview of how saliency maps are used to generate explanations in the literature. In this section, we give a more detailed description and provide examples.

A saliency map is an image, likely of the same size of the input one, that highlights which parts of the input image were most responsible for a particular output, revealing where the model focuses attention and possibly showing mistakes the network made in the prediction. The explanation is given either by superimposition or by masking. For the superimposition case, the generated saliency map is added to the input image by means of color-mapping: the explanation will show warmer (red) hues over regions the network deemed useful in the decision, and colder (blue) hues where the features of the images were not taken into consideration for the decision (as in Fig 3, center). For what regards masking, the original image is blacked/whitened out based on the pixel-wise saliency values. This results in an image that only shows the regions of the input that affected the model's decision (as in Fig 3, right).

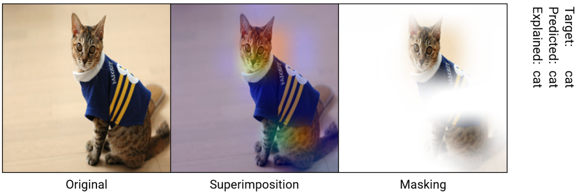


Figure 3: Different ways of displaying a saliency map for an image. The class to be explained is “cat”.

# 3 Survey intro and tutorial

Both surveys present an introductory section aimed at ensuring that participants possessed a baseline knowledge level regarding the images that they were going to see. Figure 4 shows the introductory tutorial that was presented to the subjects of our survey. This section was followed by a short example (Figure 5) to prepare users to the images they were required to evaluate during the survey.

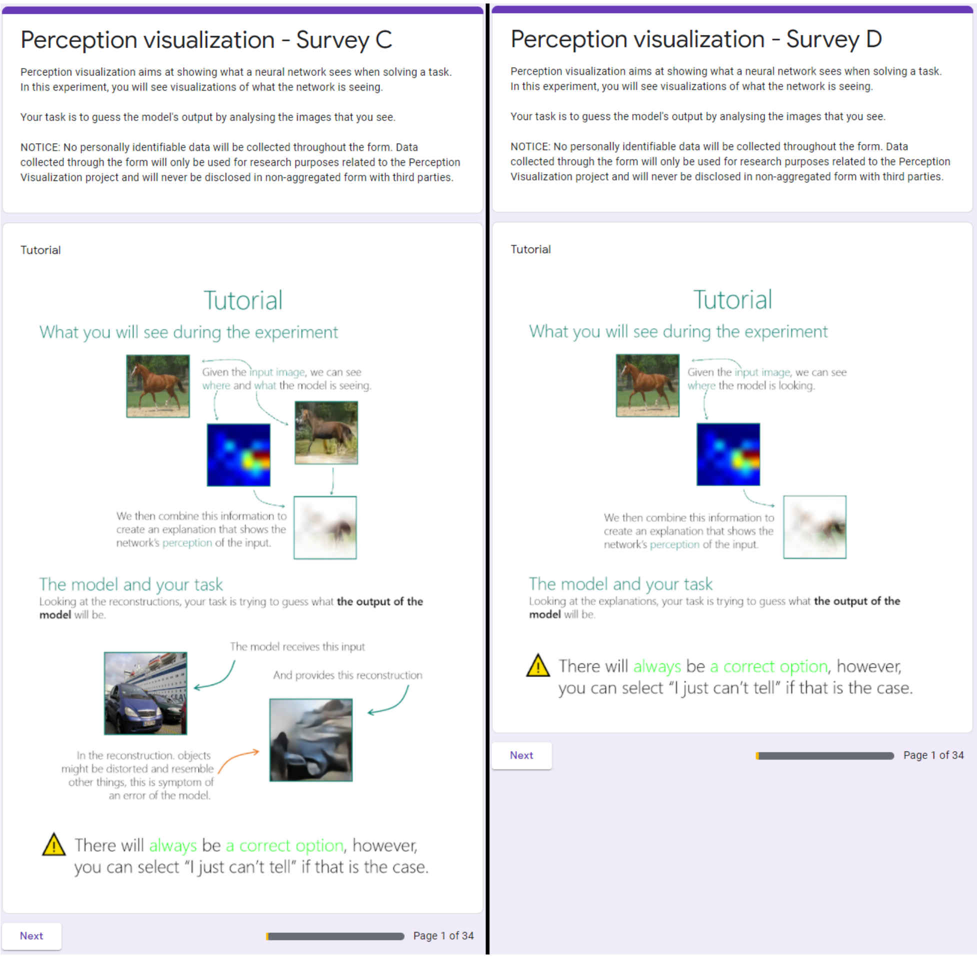


Figure 4: Tutorial page for the PV (left) and for the CAM (right) versions of the survey. This is the first page seen by users of the survey.

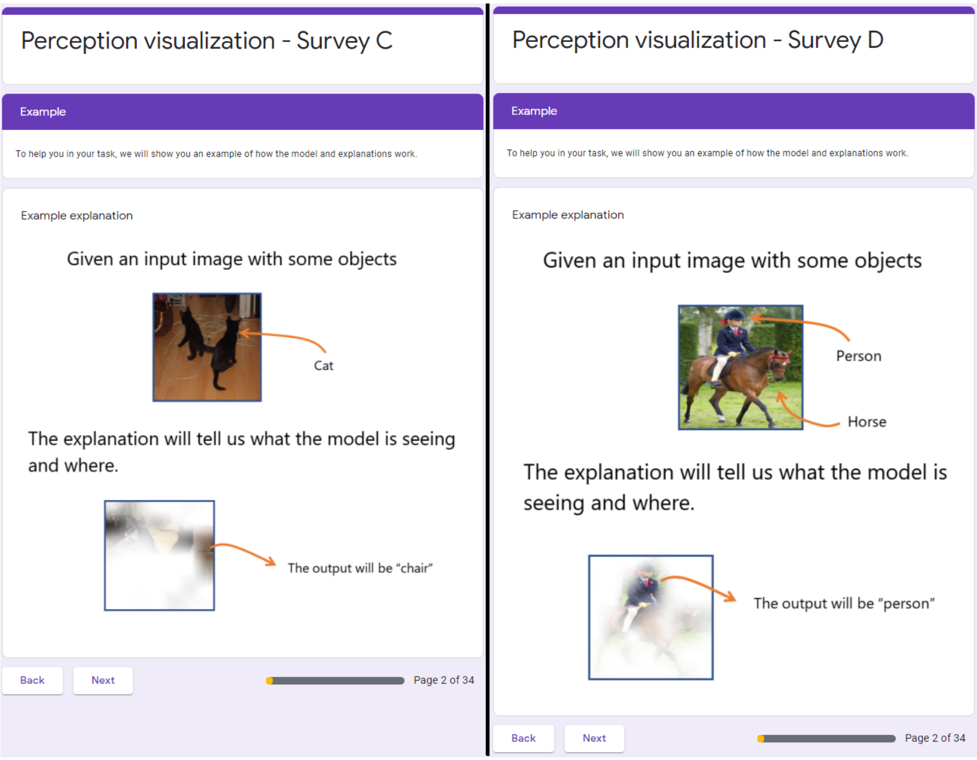


Figure 5: Example page for the PV (left) and for the CAM (right) versions of the survey. This is the second page seen by users of the survey.

# 4 Survey questions

In this section, we present all the 30 questions that were posed to the participants of our survey. For each, we show the images that were displayed in the question, the sample labels, model prediction and explained class. We also show the options that the participants could choose from and the performance of the respondents, organized by survey type (CAM/PV). An example of the data presentation is given in Figure 6.

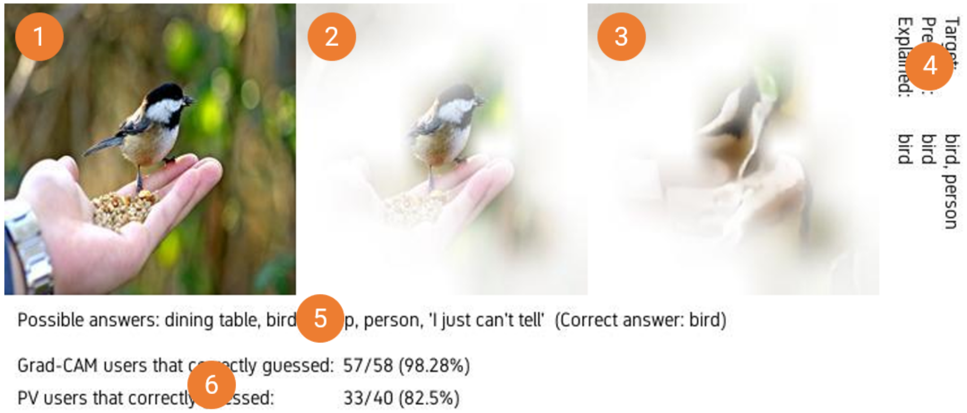


Figure 6: Overview of the data presentation. 1) The original sample, 2) The Grad-CAM explanation, 3) The PV explanation, 4) Targets, model predictions, and explained class for the specific input sample, 5) The possible answers that were given in the survey, 6) Performance of respondents for the two surveys. Participants of the CAM version of the survey see images 1 and 2, while participants of the PV version of the survey see images 1 and 3. Information 4 and 6 is hidden from the participants.

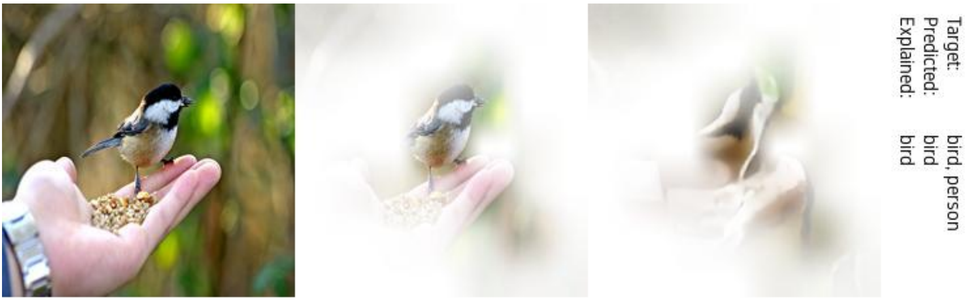


Possible answers: dining table, bird, sheep, person, 'I just can't tell' (Correct answer: bird)

Grad-CAM users that correctly guessed: 57/58 (98.28%)
PV users that correctly guessed: 33/40 (82.5%)

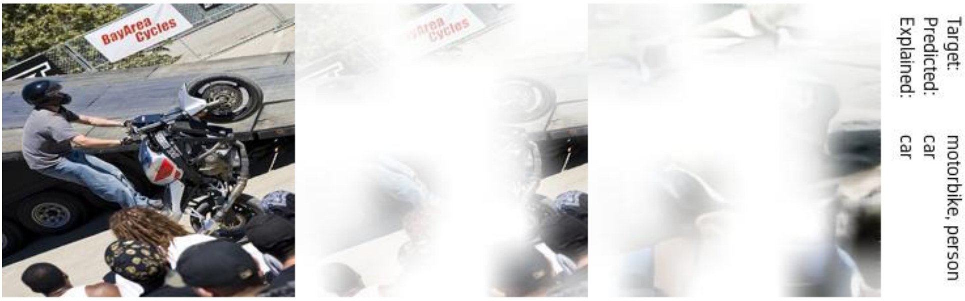


Possible answers: motorbike, car, dining table, person, 'I just can't tell' (Correct answer: car)

Grad-CAM users that correctly guessed: 0/58 (0.0%)
PV users that correctly guessed: 10/40 (25.0%)

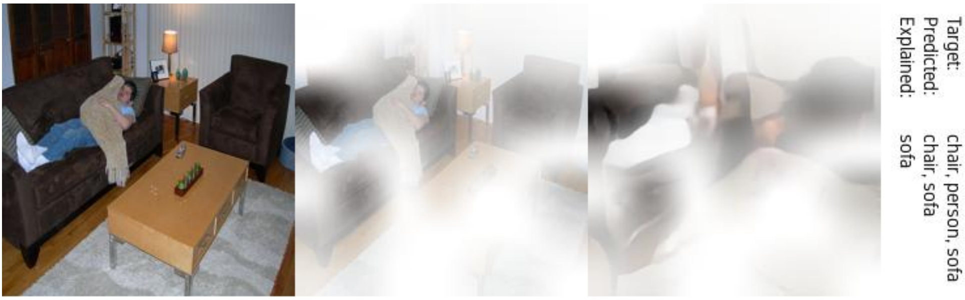


Possible answers: sofa, car, chair, person, 'I just can't tell' (Correct answer: sofa)

Grad-CAM users that correctly guessed: 3/58 (5.17%)
PV users that correctly guessed: 36/40 (90.0%)

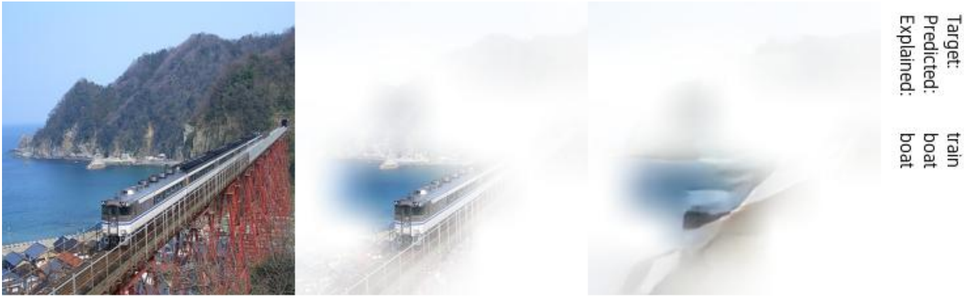


Possible answers: horse, person, train, boat, 'I just can't tell' (Correct answer: boat)

Grad-CAM users that correctly guessed: 10/58 (17.24%)
PV users that correctly guessed: 30/40 (75.0%)

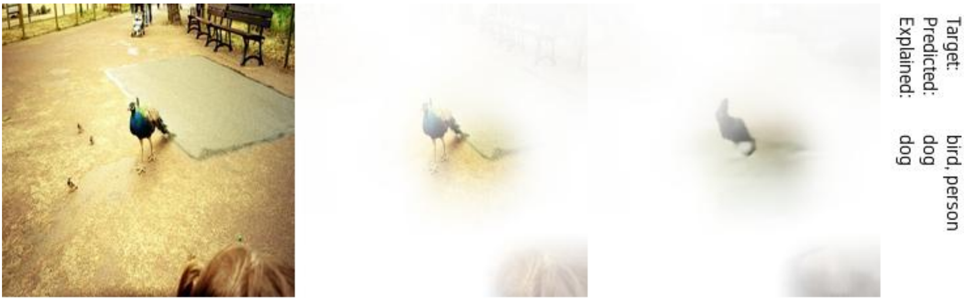


Possible answers: dog, aeroplane, bird, person, 'I just can't tell' (Correct answer: dog)

Grad-CAM users that correctly guessed: 0/58 (0.0%)
PV users that correctly guessed: 3/40 (7.5%)

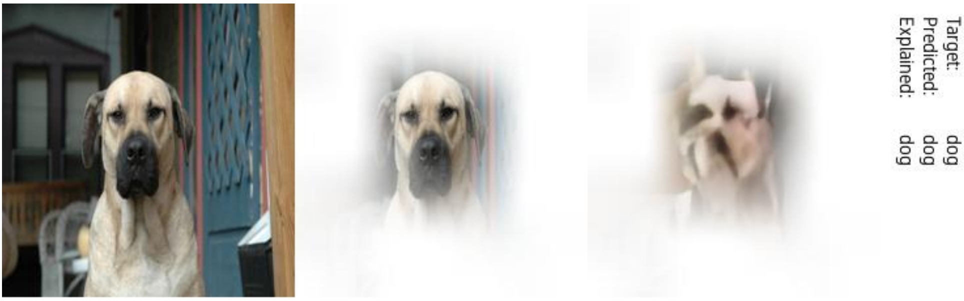


Possible answers: dog, horse, cow, bottle, 'I just can't tell' (Correct answer: dog)

Grad-CAM users that correctly guessed: 58/58 (100.0%)
PV users that correctly guessed: 32/40 (80.0%)

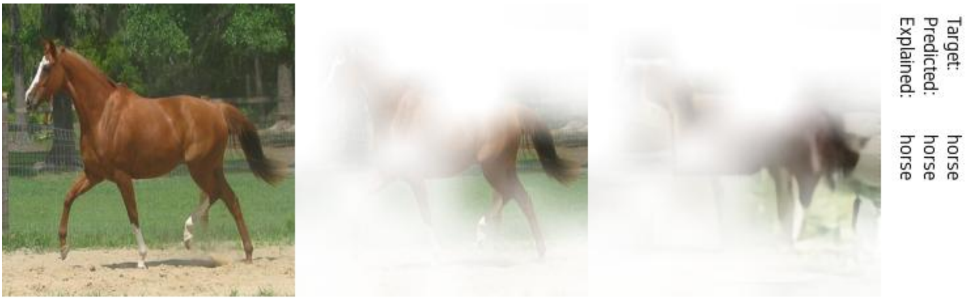


Possible answers: dog, horse, train, car, 'I just can't tell' (Correct answer: horse)

Grad-CAM users that correctly guessed: 47/58 (81.03%)
PV users that correctly guessed: 34/40 (85.0%)

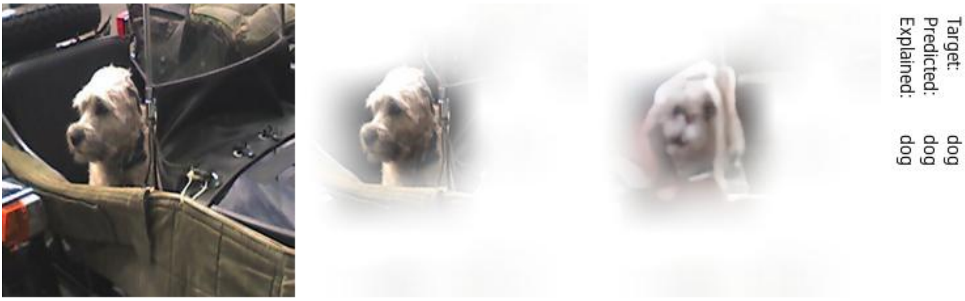


Possible answers: dog, cat, bird, train, 'I just can't tell' (Correct answer: dog)

Grad-CAM users that correctly guessed: 58/58 (100.0%)
PV users that correctly guessed: 29/40 (72.5%)

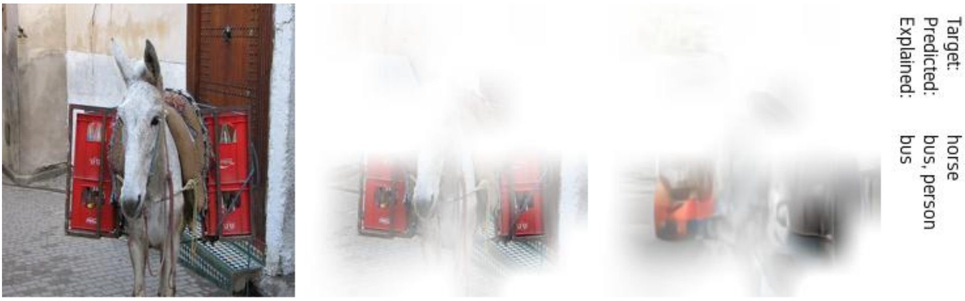


Possible answers: bus, motorbike, horse, potted plant, 'I just can't tell' (Correct answer: bus)

Grad-CAM users that correctly guessed: 13/58 (22.41%)
PV users that correctly guessed: 13/40 (32.5%)

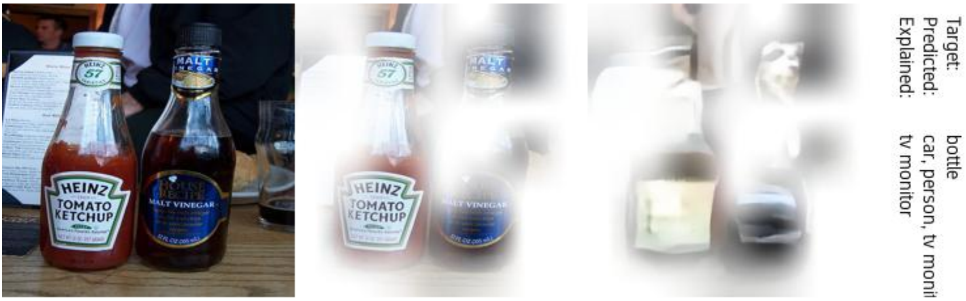


Possible answers: cow, dining table, tv monitor, bottle, 'I just can't tell' (Correct answer: tv monitor)

Grad-CAM users that correctly guessed: 1/58 (1.72%)

PV users that correctly guessed: 13/40 (32.5%)

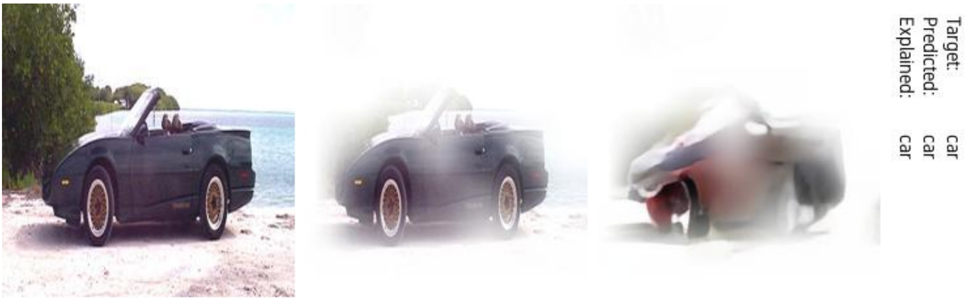


Possible answers: car, aeroplane, sheep, person, 'I just can't tell' (Correct answer: car)

Grad-CAM users that correctly guessed: 57/58 (98.28%)

PV users that correctly guessed: 29/40 (72.5%)

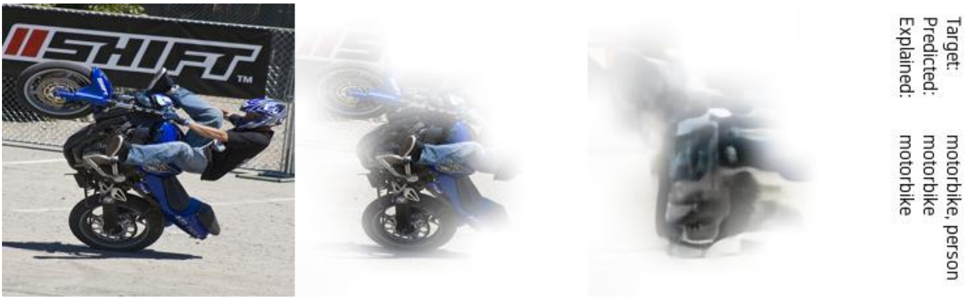


Possible answers: motorbike, car, boat, person, 'I just can't tell' (Correct answer: motorbike)

Grad-CAM users that correctly guessed: 58/58 (100.0%)

PV users that correctly guessed: 27/40 (67.5%)

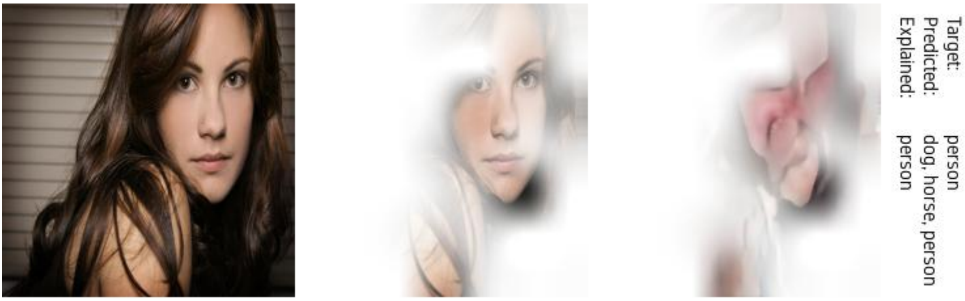


Possible answers: sofa, sheep, train, person, 'I just can't tell' (Correct answer: person)

Grad-CAM users that correctly guessed: 58/58 (100.0%)
PV users that correctly guessed: 25/40 (62.5%)

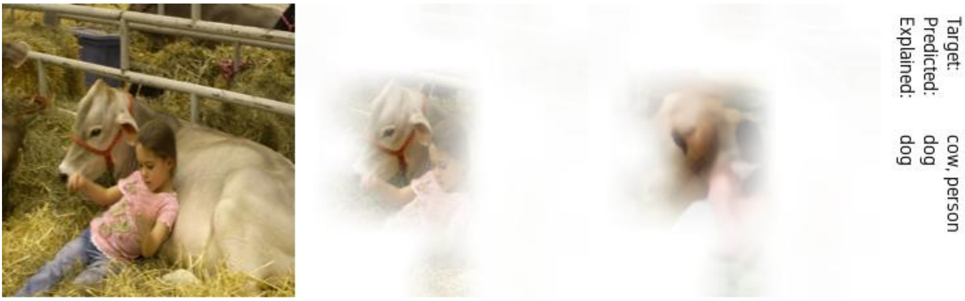


Possible answers: dog, cow, cat, person, 'I just can't tell' (Correct answer: dog)

Grad-CAM users that correctly guessed: 3/58 (5.17%)
PV users that correctly guessed: 17/40 (42.5%)

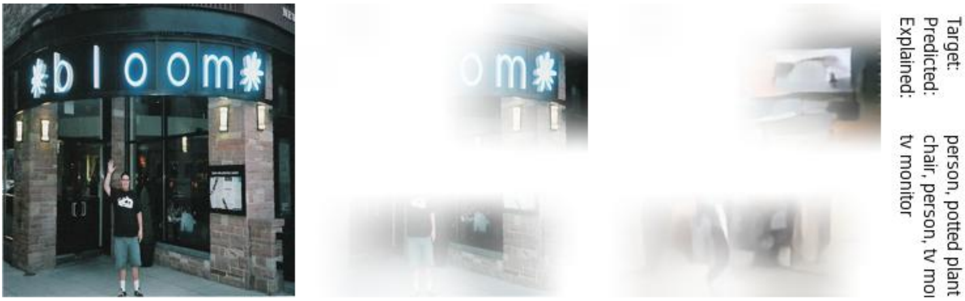


Possible answers: potted plant, cow, tv monitor, person, 'I just can't tell' (Correct answer: tv monitor)

Grad-CAM users that correctly guessed: 12/58 (20.69%)
PV users that correctly guessed: 31/40 (77.5%)

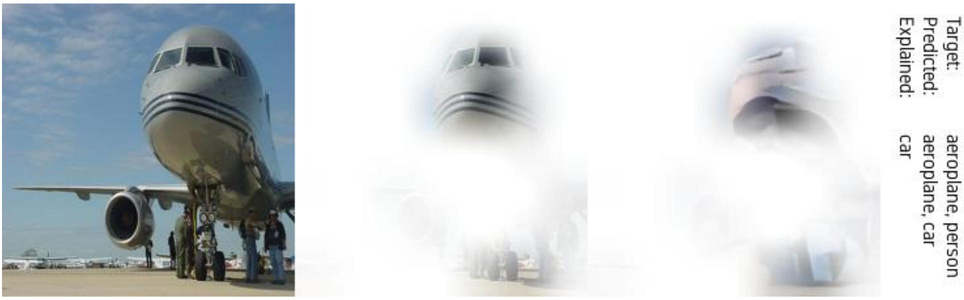


Possible answers: car, aeroplane, chair, person, 'I just can't tell' (Correct answer: car)

Grad-CAM users that correctly guessed: 0/58 (0.0%)

PV users that correctly guessed: 1/40 (2.5%)

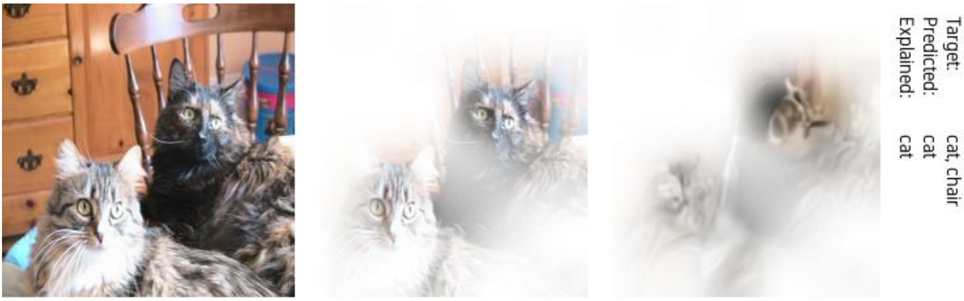


Possible answers: cat, bird, chair, bottle, 'I just can't tell' (Correct answer: cat)

Grad-CAM users that correctly guessed: 58/58 (100.0%)

PV users that correctly guessed: 38/40 (95.0%)

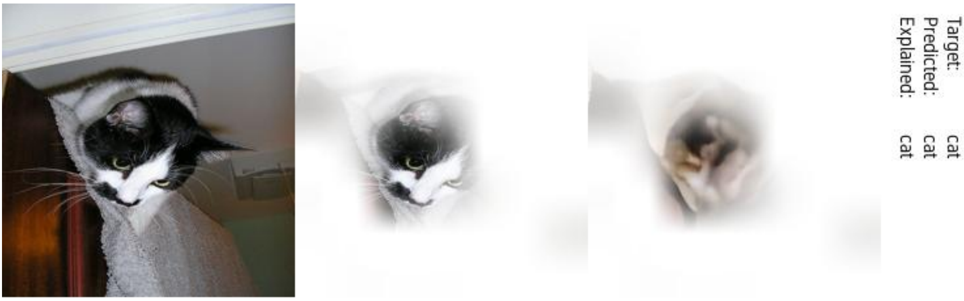


Possible answers: dog, potted plant, cat, aeroplane, 'I just can't tell' (Correct answer: cat)

Grad-CAM users that correctly guessed: 57/58 (98.28%)

PV users that correctly guessed: 32/40 (80.0%)

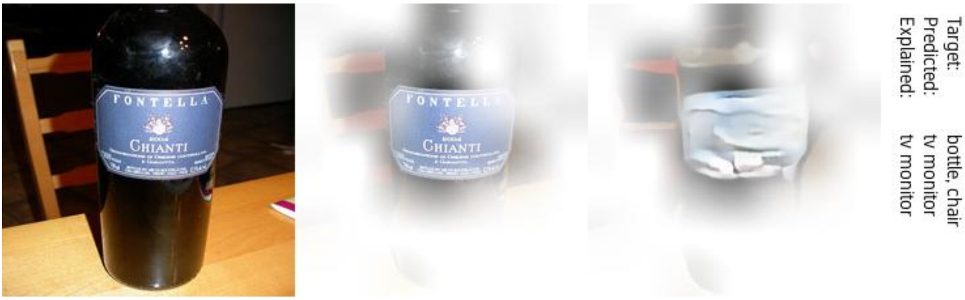


Possible answers: motorbike, chair, tv monitor, bottle, 'I just can't tell' (Correct answer: tv monitor)

Grad-CAM users that correctly guessed: 3/58 (5.17%)
PV users that correctly guessed: 17/40 (42.5%)

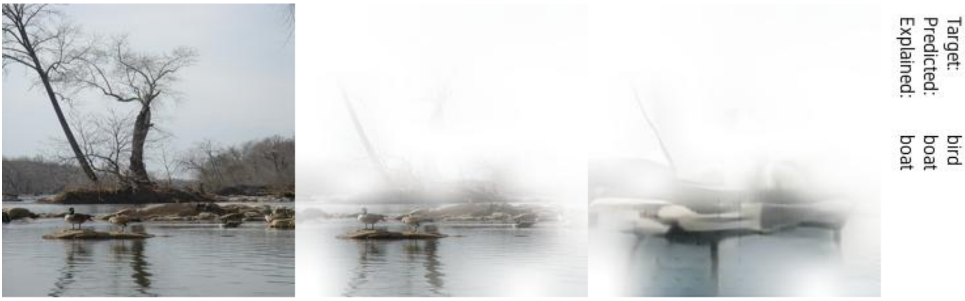


Possible answers: aeroplane, bird, train, boat, 'I just can't tell' (Correct answer: boat)

Grad-CAM users that correctly guessed: 17/58 (29.31%)
PV users that correctly guessed: 31/40 (77.5%)

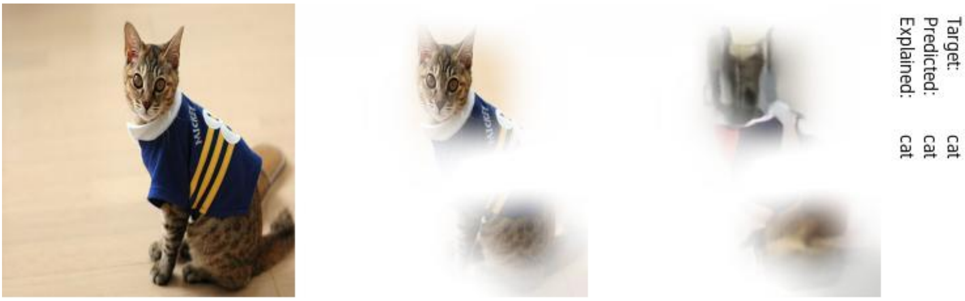


Possible answers: cat, bird, bicycle, tv monitor, 'I just can't tell' (Correct answer: cat)

Grad-CAM users that correctly guessed: 58/58 (100.0%)
PV users that correctly guessed: 19/40 (47.5%)

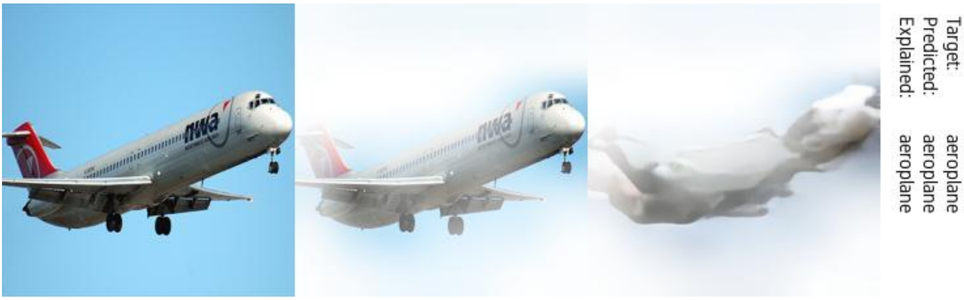


Possible answers: motorbike, aeroplane, bicycle, boat, 'I just can't tell' (Correct answer: aeroplane)

Grad-CAM users that correctly guessed: 58/58 (100.0%)
PV users that correctly guessed: 38/40 (95.0%)

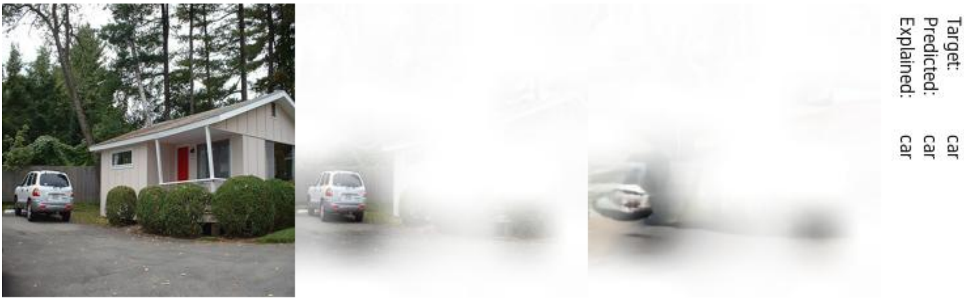


Possible answers: car, cat, aeroplane, train, 'I just can't tell' (Correct answer: car)

Grad-CAM users that correctly guessed: 58/58 (100.0%)
PV users that correctly guessed: 28/40 (70.0%)

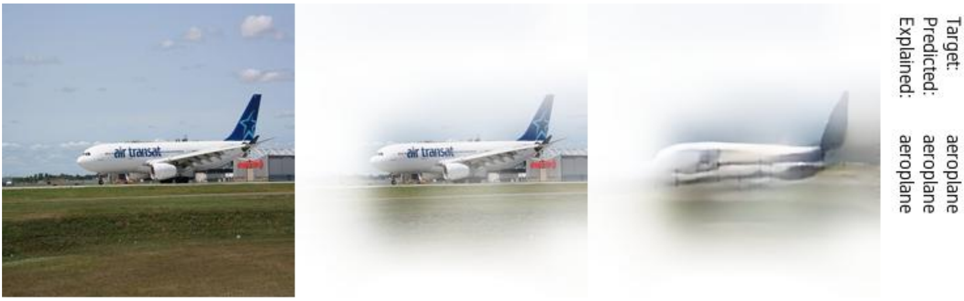


Possible answers: motorbike, potted plant, aeroplane, bicycle, 'I just can't tell' (Correct answer: aeroplane)

Grad-CAM users that correctly guessed: 58/58 (100.0%)
PV users that correctly guessed: 41/40 (102.5%)

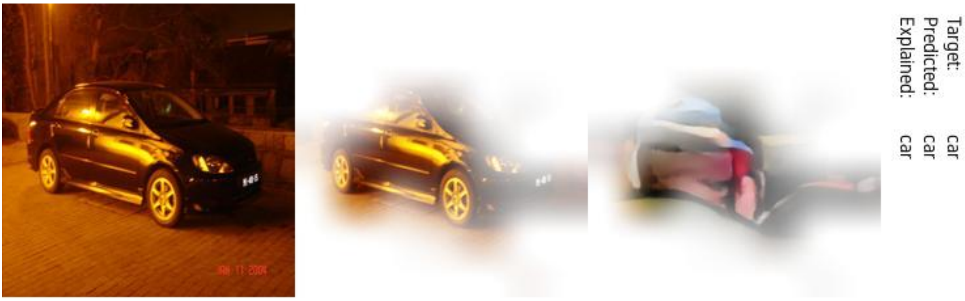


Possible answers: car, horse, dining table, chair, 'I just can't tell' (Correct answer: car)

Grad-CAM users that correctly guessed: 58/58 (100.0%)
PV users that correctly guessed: 28/40 (70.0%)

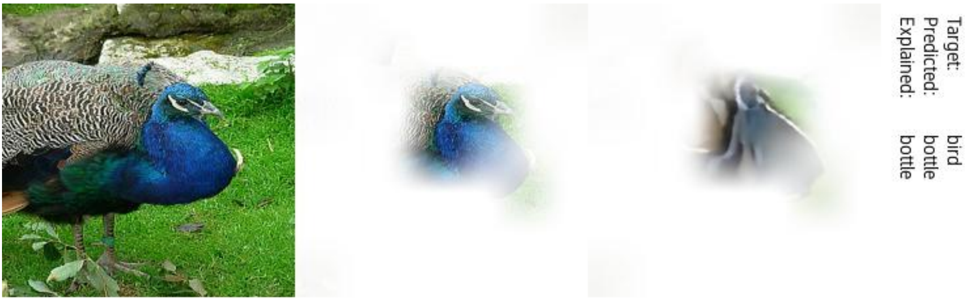


Possible answers: cow, bird, bicycle, bottle, 'I just can't tell' (Correct answer: bottle)

Grad-CAM users that correctly guessed: 1/58 (1.72%)
PV users that correctly guessed: 4/40 (10.0%)

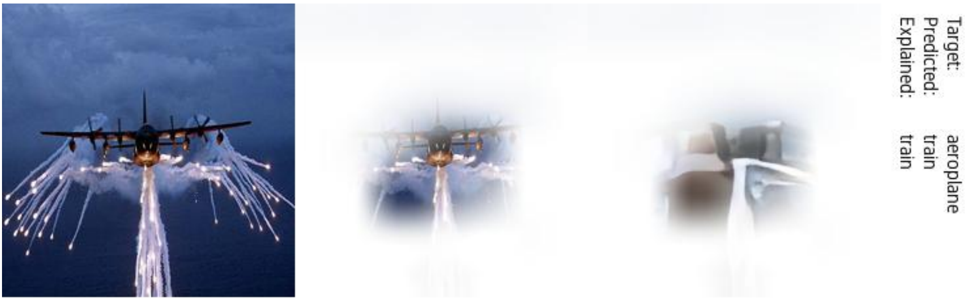


Possible answers: aeroplane, train, tv monitor, person, 'I just can't tell' (Correct answer: train)

Grad-CAM users that correctly guessed: 2/58 (3.45%)
PV users that correctly guessed: 15/40 (37.5%)

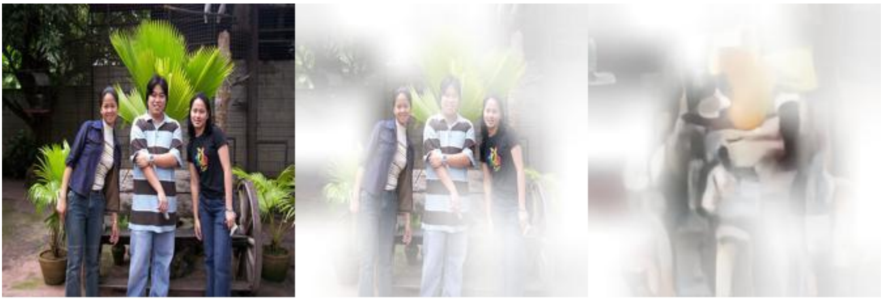


Possible answers: potted plant, aeroplane, bird, person, 'I just can't tell' (Correct answer: person)

Grad-CAM users that correctly guessed: 54/58 (93.1%)

PV users that correctly guessed: 30/40 (75.0%)

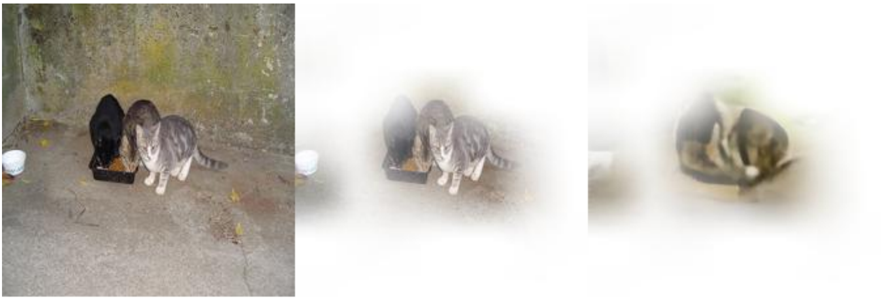


Possible answers: dog, horse, cat, person, 'I just can't tell' (Correct answer: dog)

Grad-CAM users that correctly guessed: 1/58 (1.72%)

PV users that correctly guessed: 5/40 (12.5%)

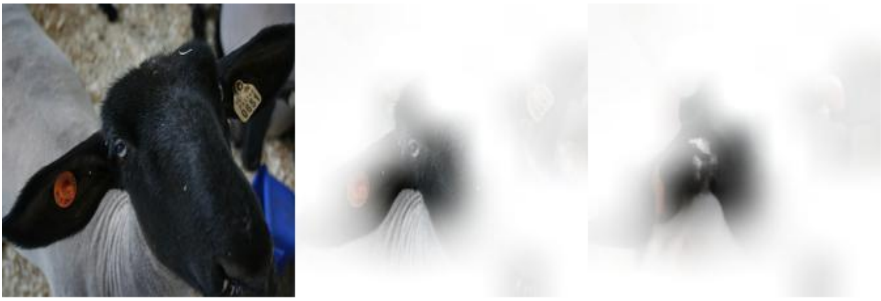


Possible answers: sofa, dog, sheep, tv monitor, 'I just can't tell' (Correct answer: dog)

Grad-CAM users that correctly guessed: 4/58 (6.9%)

PV users that correctly guessed: 7/40 (17.5%)

# References

[1] Martin Arjovsky, Soumith Chintala, and Léon Bottou. Wasserstein generative adversarial networks. In *International conference on machine learning*, pages 214–223. PMLR, 2017.

[2] Alexey Dosovitskiy and Thomas Brox. Generating images with perceptual similarity metrics based on deep networks. *arXiv preprint arXiv:1602.02644*, 2016.

[3] Ishaan Gulrajani, Faruk Ahmed, Martin Arjovsky, Vincent Dumoulin, and Aaron Courville. Improved training of wasserstein gans. *arXiv preprint arXiv:1704.00028*, 2017.

[4] Jonathan Long, Evan Shelhamer, and Trevor Darrell. Fully convolutional networks for semantic segmentation. In *Proceedings of the IEEE conference on computer vision and pattern recognition*, pages 3431–3440, 2015.

[5] Aravindh Mahendran and Andrea Vedaldi. Visualizing deep convolutional neural networks using natural pre-images. *International Journal of Computer Vision*, 120(3):233–255, 2016.

[6] Olaf Ronneberger, Philipp Fischer, and Thomas Brox. U-net: Convolutional networks for biomedical image segmentation. In *International Conference on Medical image computing and computer-assisted intervention*, pages 234–241. Springer, 2015.
